# Supplementary material for: Randomized Local Model Order Reduction
Source: arXiv:1706.09179 ancillary file (2018-03-21)
Supplement: Supplementary file 1 [file supplementary_materials.pdf]

# SUPPLEMENTARY MATERIALS: RANDOMIZED LOCAL MODEL ORDER REDUCTION*

ANDREAS BUHR† AND KATHRIN SMETANA‡

**SM1. Caccioppoli inequality.** We state the Caccioppoli inequality in this section exemplarily for the equation of heat conduction. To that end we consider on $\Omega$ the following partial differential equation (PDE)

$$-\operatorname{div}(k\nabla u) = 0 \quad \text{in } \mathcal{X}_0' \text{ for } u \in H^1(\Omega), \tag{SM1.1}$$

where $\mathcal{X}_0'$ is the dual space of $\mathcal{X}_0 := \{v \in H^1(\Omega) : v|_{\Gamma_{out}} = 0, v|_{\Sigma_D \cap \partial\Omega} = 0\}$ and $k \in L^\infty(\Omega)$ with $0 < k_0 \leq k \leq k_1 < \infty$. Alternatively, we may state for $u \in H^1(\Omega)$ the weak form as follows

$$\int_\Omega k\nabla u \nabla v \, dx = 0 \qquad \forall v \in \mathcal{X}_0. \tag{SM1.2}$$

For solutions $u$ of (SM1.2) the Caccioppoli inequality applies as stated in the following lemma.

LEMMA SM1.1 (Caccioppoli inequality). *Let $u \in H^1(\Omega)$ satisfy (SM1.2). Then, on $\Omega^* \subsetneq \Omega^{**} \subset \Omega$ with $\operatorname{dist}(\partial\Omega^* \setminus \partial\Omega, \partial\Omega^{**} \setminus \partial\Omega) > \varrho > 0$ there holds*

$$\left(\int_{\Omega^*} k|\nabla u|^2 \, dx\right)^{1/2} \leq \frac{2c\sqrt{k_1}}{\varrho}\|u\|_{L^2(\Omega^{**}\setminus\Omega^*)} \leq \frac{2c\sqrt{k_1}}{\varrho}\|u\|_{L^2(\Omega)}, \tag{SM1.3}$$

*where $c$ depends on the geometry of $\Omega$.*

*Proof.* The proof follows the lines of the proof of [SM2, Theorem 4.1]. We define a cut-off function $\zeta \in C^1(\Omega) \cap C^0(\overline{\Omega})$ with $0 \leq \zeta \leq 1$ on $\Omega$, $\zeta \equiv 1$ on $\Omega^*$ and $\zeta \equiv 0$ on $\Omega \setminus \Omega^{**}$, and $|\nabla\zeta(x)| \leq c/\varrho$ on $\Omega$. By using $\zeta^2 u$ as a test function in (SM1.2) we obtain

$$\int_\Omega k\zeta^2 \nabla u \nabla u \, dx + 2\int_\Omega ku\zeta\nabla u \nabla\zeta \, dx = \int_\Omega k\nabla u \nabla(\zeta^2 u) \, dx = 0.$$

Applying Hölder's inequality yields

$$\int_\Omega k\zeta^2|\nabla u|^2 \, dx \leq \left(\int_\Omega k\zeta^2|\nabla u|^2 \, dx\right)^{1/2} \left(4\int_\Omega ku^2|\nabla\zeta|^2 \, dx\right)^{1/2}.$$

By exploiting the properties of $\zeta$ we may then conclude

$$\left(\int_{\Omega^*} k|\nabla u|^2 \, dx\right)^{1/2} \leq \frac{2c\sqrt{k_1}}{\varrho}\|u\|_{L^2(\Omega^{**}\setminus\Omega^*)}.$$

*Submitted to the editors July 3, 2017.
**Funding:** Andreas Buhr was supported by CST Computer Simulation Technology AG.
†Institute for Computational and Applied Mathematics, University of Münster, Einsteinstraße 62, 48149 Münster, Germany. (andreas@andreasbuhr.de).
‡Institute for Computational and Applied Mathematics, University of Münster, Einsteinstraße 62, 48149 Münster, Germany; current address: Department of Applied Mathematics, University of Twente, P.O. Box 217, 7500 AE Enschede, The Netherlands. (k.smetana@utwente.nl).

□

The Caccioppoli inequality can be shown for elliptic PDEs. For the proof for elliptic systems we refer to [SM2, Theorem 4.1] and for Helmholtz's equation, elastodynamics, and Stokes' problem see for instance [SM8].

**SM2. Analytical Example.** The problem used in subsection 4.1 can be solved analytically. We consider the problem $\mathcal{A} = -\Delta$, $f = 0$, and assume that $\Omega = (-L, L) \times (0, W)$, $\Gamma_{out} = \{-L, L\} \times (0, W)$, and $\Gamma_{in} = \{0\} \times (0, W)$. Moreover, we prescribe homogeneous Neumann boundary conditions on $\partial\Omega \setminus \Gamma_{out}$ and arbitrary Dirichlet boundary conditions on $\Gamma_{out}$. We may then proceed with separation of variables and deduce that all $\mathcal{A}$-harmonic functions, i.e. all solutions of this problem, are of the form

$$u(x_1, x_2) = a_0 + b_0 x_1 + \sum_{n=1}^{\infty} \cos(n\pi \frac{x_2}{W}) \left[ a_n \cosh(n\pi \frac{x_1}{W}) + b_n \sinh(n\pi \frac{x_1}{W}) \right], \tag{SM2.1}$$

where $x_1 \in (-L, L)$, $x_2 \in (0, W)$, and the coefficients $a_n, b_n \in \mathbb{R}$, $n = 0, \ldots, \infty$ are determined by the Dirichlet data on $\Gamma_{out}$. Thanks to the behavior of the cosh function we observe a very rapid and in fact exponential decay of the $\mathcal{A}$-harmonic functions (SM2.1) from $\Gamma_{out}$ to the interior of $\Omega$. As most of the $\mathcal{A}$-harmonic functions (SM2.1) have therefore negligibly small values on $\Gamma_{in}$, we anticipate that already a reduced space of very low dimension will yield an accurate approximation of all $\mathcal{A}$-harmonic functions (SM2.1).

For many situations an exponential convergence of the eigenvalues of the transfer eigenproblem (2.6) and the respective domain decomposition or multiscale approximations can be observed (see section 4). For this example we have $\lambda_j = (\cosh((L(j-1)\pi)/H))^{-2}$, $j = 1, 2, \ldots$ if we use an inner product that is defined via $\mathcal{A}$-harmonic extensions of functions on $\Gamma_{in}$ and $\Gamma_{out}$.

**SM3. Proof of Theorem 3.3.** *Proof.* We give here only the main ideas for the proof to explain the origin of the occurring terms and refer for details to [SM6]. Let $\underline{T} = \underline{U\Sigma V}^t$ be the SVD of $\underline{T}$. Then, we denote the matrix which contains the largest $n$ singular values on the diagonal as $\underline{\Sigma}_1$ and the matrix with the remaining singular values on the diagonal as $\underline{\Sigma}_2$. Next, we define $\underline{V}_1^t$ as the submatrix that contains the first $n$ rows of $\underline{V}^t$ and $\underline{V}_2^t$ as the submatrix containing the remaining rows. Let finally $\underline{\Upsilon}$ denote a test matrix and define $\underline{\Upsilon}_1 = \underline{V}_1^t \underline{\Upsilon}$ and $\underline{\Upsilon}_2 = \underline{V}_2^t \underline{\Upsilon}$. If $\underline{\Upsilon}_1$ has full row rank one may then prove with arguments inspired by perturbation theory of orthogonal projectors (see [SM6, Theorem 9.1] for details) that there holds

$$\|\underline{T} - \underline{P}_{R^n,2}\underline{T}\|^2 \leq \|\underline{\Sigma}_2\|^2 + \|\underline{\Sigma}_2 \underline{\Upsilon}_2 \underline{\Upsilon}_1^+\|^2, \tag{SM3.1}$$

where $\underline{\Upsilon}_1^+$ is the pseudoinverse of $\underline{\Upsilon}_1$. To derive a bound for the expected value of the last term in (SM3.1) for standard Gaussian test matrices $\underline{\Upsilon}$ Halko et al. employ the following inequality that is due to Gordon [SM4, SM5] and has been shown by using a sharp bound of Slepian's lemma:

$$\mathbb{E}(\|\underline{A\Upsilon B}\|) \leq \|\underline{A}\|\|\underline{B}\|_F + \|\underline{A}\|_F\|\underline{B}\|. \tag{SM3.2}$$

Here, $\underline{A}$ and $\underline{B}$ are fixed real matrices and $\|\cdot\|_F$ denotes the Frobenius norm. By using the bound in [SM1, Lemma 4.1] on the probability that the spectral norm of the pseudoinverse of a Gaussian matrix is large and applying Stirling's approximation we obtain that $\mathbb{E}(\|\underline{\Upsilon}_1^+\|) < (e\sqrt{n})/p$. Finally, Halko et al employ that the squared

Frobenius norm of a pseudoinverted Gaussian matrix equals the trace of an inverted Wishart matrix. As the diagonal of the latter consists of inverted $\chi^2$ variates [SM6, Proposition A.5], we obtain $\mathbb{E}(\|\underline{\Upsilon}_1^+\|_F^2) = k/(p-1)$ [SM6, Proposition A.6], which concludes the (outline of the) proof. ∎

**SM4. Improved Estimates.** By multiplying the random normal vectors with the inverse square root of the inner product matrix in $S$ before applying the transfer operator, better estimates can be optained.

LEMMA SM4.1 (Distribution of inner product). *The inner product of a normed vector $v$ in $S$ with a the product of the inverse square root of the inner product matrix in $S$ and a random normal vector $(v, D_S^{-1}\underline{M}_S^{-1/2}\underline{r})_S$ is a Gaussian distributed random variable with mean zero and variance one.*

*Proof.* We use the spectral decomposition of the inner product matrix $\underline{M}_S = \sum_{i=1}^{N_S} \underline{m}_{S,i}\lambda_i^{M_S}\underline{m}_{S,i}^T$ and $\underline{M}_S^{-1/2} = \sum_{i=1}^{N_S} \underline{m}_{S,i}\left(\lambda_i^{M_S}\right)^{-1/2}\underline{m}_{S,i}^T$ with eigenvalues $\lambda_i^{M_S}$ and eigenvectors $\underline{m}_{S,i}$. There holds

$$(v, D_S^{-1}\underline{M}_S^{-1/2}\underline{r})_S = \sum_{i=1}^{N_S}(D_S v)^T \underline{m}_{S,i}\left(\lambda_i^{M_S}\right)^{1/2}\underline{m}_{S,i}^T\underline{r}. \tag{SM4.1}$$

As $m_{S,i}$ is normed with respect to the euclidean inner product, the term $\underline{m}_{S,i}^T\underline{r}$ is a normal distributed random variable. Using the rules for addition and scalar multiplication of Gaussian random variables, one sees that the inner product $(v, D_S^{-1}\underline{M}_S^{-1/2}\underline{r})_S$ is a Gaussian random variable with variance 1.

$$\sum_{i=1}^{N_S}\left((D_S v)^T\underline{m}_{S,i}\left(\lambda_i^{M_S}\right)^{1/2}\right)^2 = 1. \tag{SM4.2}$$

∎

PROPOSITION SM4.2 (Improved a priori estimate). *If we use $TD_S^{-1}\underline{M}_S^{-1/2}\underline{r}$ instead of $TD_S^{-1}\underline{r}$ in Algorithm 1 to generate basis vectors and test vectors, the a priori estimates in Proposition 3.2 hold without the factor $(\lambda_{max}^{M_S}/\lambda_{min}^{M_S})^{1/2}$.*

*Proof.* Only slight modifications of the proofs are required. In the third line of the proof of Lemma 3.4 we exploit the bijectivity of $\underline{M}_S^{-1/2}$ and substitute $\underline{\xi} = \underline{M}_S^{-1/2}\underline{\zeta}$ to arrive at $\|T - P_{R^n}T\| \leq (\lambda_{max}^{M_R})^{1/2}\|\underline{TM}_S^{-1/2} - \underline{P}_{R^n,2}\underline{TM}_S^{-1/2}\|_2$. Moreover, we bound the singular values $\underline{\sigma}_j^M$ of $\underline{TM}_S^{-1/2}$ by the singular values $\sigma_j$ of the operator $T$: $\underline{\sigma}_j^M \leq (\lambda_{min}^{M_R})^{-1/2}\sigma_j$. To that end, the Courant minimax principle has to be employed only once in the proof of Lemma 3.5. Combining these bounds with the estimates in Theorem 3.3 yields the estimates in Proposition 3.2 without the factor $(\lambda_{max}^{M_S}/\lambda_{min}^{M_S})^{1/2}$. ∎

PROPOSITION SM4.3 (Improved norm estimator). *If we define the error estimator as*

$$\Delta^M(O, n_t, \varepsilon_{\mathrm{testfail}}) := c_{\mathrm{est}}^M(n_t, \varepsilon_{\mathrm{testfail}}) \max_{i\in 1,\dots,n_t}\left\|O\ D_S^{-1}\ \underline{M}_S^{-1/2}\ \underline{r}_i\right\|_R, \tag{SM4.3}$$

*with $c_{\mathrm{est}}^M(n_t, \varepsilon_{\mathrm{testfail}}) := \left[\sqrt{2}\,\mathrm{erf}^{-1}\left(\sqrt[n_t]{\varepsilon_{\mathrm{testfail}}}\right)\right]^{-1}$, Proposition 3.7 still holds true:*

$P\Big(\|O\| \leq \Delta^M(O, n_t, \varepsilon_{\text{testfail}})\Big) \geq 1 - \varepsilon_{\text{testfail}}$. *Additionally, we have*

$$P\left(\frac{\Delta^M(O, n_t, \varepsilon_{\text{testfail}})}{\|O\|} \leq c^M_{\text{eff}}(n_t, \varepsilon_{\text{testfail}})\right) \geq 1 - \varepsilon_{\text{testfail}}$$

*with*

$$c^M_{\text{eff}}(n_t, \varepsilon_{\text{testfail}}) := \left[Q^{-1}\left(\frac{N_O}{2}, \frac{\varepsilon_{\text{testfail}}}{n_t}\right)\left(\text{erf}^{-1}\left(\sqrt[n_t]{\varepsilon_{\text{testfail}}}\right)\right)^{-2}\right]^{1/2}.$$

*Proof.* Only slight modifications to the proofs of Propositions 3.7 and 3.8 are required: (1) $D_S^{-1}\underline{r}$ has to be replaced by $D_S^{-1}\underline{M_S}^{-1/2}\underline{r}$, (2) $c_{\text{eff}}$ has to be replaced by $c^M_{\text{eff}}$, (3) $c_{\text{est}}$ has to be replaced by $c^M_{\text{est}}$, (4) $\lambda^{\underline{M_S}}_{min}$ and $\lambda^{\underline{M_S}}_{max}$ have to be replaced by 1. ◻

While the a priori estimates are better when using $TD_S^{-1}\underline{M_S}^{-1/2}\underline{r}$ instead of $TD_S^{-1}\underline{r}$ in Algorithm 1, we concentrate on the usage of $TD_S^{-1}\underline{r}$ in this publication as the application of the inverse square root may be computationally expensive.

## SM5. GFEM.

**SM5.1. Algorithm.** The full GFEM algorithm is given in Algorithm 1.

**SM5.2. GFEM Convergence.** In this section, we establish error bounds for the GFEM with randomized basis generation. The error of the GFEM solution with respect to the full FEM solution is lower than a prescribed tolerance $\texttt{tol}_{\text{GFEM}}$. There are no unknown constants in the procedure. We first show in Proposition SM5.1 that the relative global error can be bounded by the local relative approximation errors. Then in Lemma SM5.2 we establish that the local relative approximation error can be bounded when the local spaces are constructed using the presented randomized algorithm. Finally we combine these results in Corollary SM5.3 and give an error bound for the GFEM with randomized basis generation.

We require a partition of unity $\{\varrho_i\}_{i=1}^m$ subordinate to the open cover $\{\omega_i\}_{i=1}^m$ satisfying

$$\varrho_i \in C^{0,1}(\omega_i), \quad i = 1, \ldots, m, \tag{SM5.1}$$

$$\operatorname{supp} \varrho_i \subset \bar{\omega}_i, \quad i = 1, \ldots, m, \tag{SM5.2}$$

$$\sum_{i=1}^m \varrho_i \equiv 1 \quad \text{on } \Omega_{gl}, \tag{SM5.3}$$

$$\|\varrho_i\|_{L^\infty(\Omega_{gl})} \leq C_1, \quad i = 1, \ldots, m, \tag{SM5.4}$$

$$\|\nabla\varrho_i\|_{L^\infty(\Omega_{gl})} \leq \frac{C_2}{\text{diam}(\omega_i)}, \quad i = 1, \ldots, m, \tag{SM5.5}$$

where $0 < C_1, C_2 < \infty$.

Moreover, we require that the open cover $\{\omega_i\}_{i=1}^m$ satisfies a pointwise overlap condition

$$\exists M \in \mathbb{N} \quad \forall x \in \Omega_{gl} \quad \text{card}\{i \,|\, x \in \omega_i\} \leq M. \tag{SM5.6}$$

Also for the domains $\omega_i^*$ we require a pointwise overlap condition:

$$\exists M^* \in \mathbb{N} \quad \forall x \in \Omega_{gl} \quad \text{card}\{i \,|\, x \in \omega_i^*\} \leq M^*. \tag{SM5.7}$$

**Algorithm 1:** GFEM

**Function** $\texttt{GFEM}(\texttt{tol}_{\text{GFEM}}, \varepsilon_{\text{fail}}, n)$**:**

**Input :** target accuracy $\texttt{tol}_{\text{GFEM}}$,
maximum failure probability $\varepsilon_{\text{fail}}$,
number of test vectors $n_t$

**Output:** approximation $u_{\text{GFEM}}$ with property

$$P\left(\frac{\|k^{1/2}\nabla(u_{gl}-u_{\text{GFEM}})\|_{L^2(\Omega_{gl})}}{\|k^{1/2}\nabla u_{gl}\|_{L^2(\Omega_{gl})}} \leq \texttt{tol}_{\text{GFEM}}\right) \geq (1-\varepsilon_{\text{fail}})$$

**for** $i \in 1, \dots, m$ **do**

`/* calculate local target accuracy */`

calculate $C_{Q,i}$

$\varepsilon_i \leftarrow \texttt{tol}_{\text{GFEM}} \left[(2MM^*)\left(\left(\frac{C_2}{\text{diam}(\omega_i)}\right)^2 C_{Q,i}^2 + C_1^2\right)\right]^{-\frac{1}{2}}$

`/* choose target operator norm */`

calculate $C_{S,i}$

$\texttt{tol}_i \leftarrow \varepsilon_i / C_{S,i}$

`/* calculate this domain's share in the failure probability */`

$\varepsilon_{\text{algofail}} \leftarrow \varepsilon_{\text{fail}}/m$

`/* invoke randomized range approximation */`

$R_i^n \leftarrow \texttt{AdaptiveRangeApproximation}(T_i, \texttt{tol}_i, n_t, \varepsilon_{\text{algofail}})$

`/* enrich the reduced space with constant and` $u_i^f$ `*/`

$R_i^n \leftarrow R_i^n \oplus \text{span}(u_i^f)$

**if** $\partial\omega_i \cap \Sigma_D = \emptyset$ **then**

$R_i^n \leftarrow R_i^n \oplus \text{span}(1)$

`/* construct GFEM space */`

$X_{\text{GFEM}} \leftarrow \bigoplus_{i=1,\dots,m} \left\{ \varrho_i v_i \;\middle|\; v_i \in R_i^n \right\}$

`/* solve projected problem */`

find $u_{\text{GFEM}} \in X_{\text{GFEM}}$ so that

$-\text{div}(k\nabla u_{\text{GFEM}}) = f \quad \text{in } X'_{\text{GFEM}}$

**return** $u_{\text{GFEM}}$

PROPOSITION SM5.1. *Let the open cover* $\{\omega_i\}_{i=1}^m$ *and the partition of unity* $\{\varrho_i\}_{i=1}^m$ *be defined as above. Assume that on each subdomain* $\omega_i$ *there exists a* $v_i \in X_i$ *such that there holds*

$$\frac{\|k^{1/2}\nabla(u_{gl}-v_i)\|_{L^2(\omega_i)}}{\|k^{1/2}\nabla u_{gl}\|_{L^2(\omega_i^*)}} \leq \varepsilon_i. \tag{SM5.8}$$

*Then there exist constants* $a_{c,i}$ *so that the function* $u^N := \sum_{i=1}^m (v_i + a_{c,i})\,\varrho_i \in X_{gl}$ *satisfies*

(SM5.9)

$$\frac{\|k^{1/2}\nabla(u_{gl}-u^N)\|_{L^2(\Omega_{gl})}}{\|k^{1/2}\nabla u_{gl}\|_{L^2(\Omega_{gl})}} \leq \sqrt{2MM^*} \max_{i\in 1,\dots,m} \left(\frac{C_2^2}{\text{diam}(\omega_i)^2} C_{p,f,i}^2 \frac{k_1}{k_0} + C_1^2\right)^{1/2} \varepsilon_i,$$

*where* $C_{p,f,i}$ *is the constant in the Poincaré inequality on subdomains* $\omega_i^*$ *that satisfy*

*$\partial\omega_i^* \cap \Sigma_D = \emptyset$ and equals the constant in the Friedrichs' inequality for subdomains $\omega_i^*$ that border $\Sigma_D$.*

*Proof.* At the beginning we follow the lines of the proof of Theorem 2.1 in [SM7]. First, we exploit (SM5.3) and obtain

$$\|k^{1/2}\nabla(u_{gl}-u^N)\|^2_{L^2(\Omega_{gl})} = \|k^{1/2}\nabla\left(\sum_{i=1}^m \varrho_i\{u_{gl}-v_i-a_{c,i}\}\right)\|^2_{L^2(\Omega_{gl})}$$
$$\leq 2\|k^{1/2}\sum_{i=1}^m(\nabla\varrho_i)(u_{gl}-v_i-a_{c,i})\|^2_{L^2(\Omega_{gl})} + 2\|k^{1/2}\sum_{i=1}^m \varrho_i\nabla(u_{gl}-v_i)\|^2_{L^2(\Omega_{gl})}.$$

Thanks to the pointwise overlap condition (SM5.6) and the properties (SM5.2), (SM5.4), and (SM5.5) we may then infer

$$\|k^{1/2}\nabla(u_{gl}-u^N)\|^2_{L^2(\Omega_{gl})}$$
$$\leq 2M\sum_{i=1}^m \|k^{1/2}(\nabla\varrho_i)(u_{gl}-v_i-a_{c,i})\|^2_{L^2(\Omega_{gl})} + 2M\sum_{i=1}^m \|k^{1/2}\varrho_i\nabla(u_{gl}-v_i)\|^2_{L^2(\Omega_{gl})}$$
$$\leq 2M\sum_{i=1}^m \|k^{1/2}(\nabla\varrho_i)(u_{gl}-v_i-a_{c,i})\|^2_{L^2(\omega_i)} + 2M\sum_{i=1}^m \|k^{1/2}\varrho_i\nabla(u_{gl}-v_i)\|^2_{L^2(\omega_i)}$$
$$\leq 2M\sum_{i=1}^m \frac{C_2^2}{\mathrm{diam}(\omega_i)^2}\|k^{1/2}(u_{gl}-v_i-a_{c,i})\|^2_{L^2(\omega_i)} + 2M\sum_{i=1}^m C_1^2\|k^{1/2}\nabla(u_{gl}-v_i)\|^2_{L^2(\omega_i)}.$$

We distinguish between subdomains $\omega_i$ that satisfy $\partial\omega_i\cap\Sigma_D=\emptyset$ and subdomains that border $\Sigma_D$, starting with the former.

Choosing $a_{c,i}$ such that $a_{c,i} = |\omega_i|^{-1}\int_{\omega_i}(u_{gl}-v_i)$ allows us to apply Poicaré's inequality with a constant $c_{p,i}$ and to infer

$$\|k^{1/2}(u_{gl}-v_i-a_{c,i})\|^2_{L^2(\omega_i)} \leq c_{p,i}^2\frac{k_1}{k_0}\|k^{1/2}\nabla(u_{gl}-v_i)\|^2_{L^2(\omega_i)} \tag{SM5.10}$$
$$\leq \varepsilon_i^2 c_{p,i}^2\frac{k_1}{k_0}\|k^{1/2}\nabla u_{gl}\|^2_{L^2(\omega_i^*)}.$$

Finally, we consider subdomains $\omega_i$ that border $\Sigma_D$. As we prescribe homogeneous Dirichlet boundary conditions, we set $a_{c,i}=0$ and directly apply Friedrichs' inequality with a constant $c_{f,i}$ and obtain

$$\|k^{1/2}(u_{gl}-v_i)\|^2_{L^2(\omega_i)} \leq c_{f,i}^2\frac{k_1}{k_0}\|k^{1/2}\nabla(u_{gl}-v_i)\|^2_{L^2(\omega_i)} \leq \varepsilon_i^2 c_{f,i}^2\frac{k_1}{k_0}\|k^{1/2}\nabla u_{gl}\|^2_{L^2(\omega_i^*)}.$$

We end up at

$$\|k^{1/2}\nabla(u_{gl}-u^N)\|^2_{L^2(\Omega_{gl})}$$
$$\leq 2M\sum_{i=1}^m \frac{C_2^2}{\mathrm{diam}(\omega_i)^2}\varepsilon_i^2 C_{p,f,i}^2\frac{k_1}{k_0}\|k^{1/2}\nabla u_{gl}\|^2_{L^2(\omega_i^*)} + 2M\sum_{i=1}^m C_1^2\varepsilon_i^2\|k^{1/2}\nabla u_{gl}\|^2_{L^2(\omega_i^*)}$$
$$\leq 2M\max_{i=1,\dots,m}\left(\frac{C_2^2}{\mathrm{diam}(\omega_i)^2}\varepsilon_i^2 C_{p,f,i}^2\frac{k_1}{k_0}+C_1^2\varepsilon_i^2\right)\sum_{i=1}^m\|k^{1/2}\nabla u_{gl}\|^2_{L^2(\omega_i^*)}.$$

Exploiting the fact that at most $M^*$ domains $\omega_i^*$ have support at any given point in $\Omega_{gl}$ and thus

$$\sum_{i=1}^{m} \|k^{1/2}\nabla u_{gl}\|^2_{L^2(\omega_i^*)} \leq M^* \|k^{1/2}\nabla u_{gl}\|^2_{L^2(\Omega_{gl})}$$

concludes the proof. □

In the numerical experiments, we do not use the constant $C^2_{p,f,i}\frac{k_1}{k_0}$ but instead introduce the constant $C_{Q,i}$ which we define as the smallest number for which

$$\|k^{1/2}v\|_{L^2(\omega_i)} \leq C_{Q,i}\|k^{1/2}\nabla v\|_{L^2(\omega_i)} \qquad \forall v \in X_{Q,i} \tag{SM5.11}$$

holds where $X_{Q,i} := X_i$ for all subdomains $\omega_i$ which have Dirichlet boundary and $X_{Q,i} := \{\varphi \in X_i\ ,\ \int_{\omega_i} k\varphi = 0\}$ for all subdomains $\omega_i$ which do not have Dirichlet boundary. Then instead of (SM5.9) it holds

$$\frac{\|k^{1/2}\nabla(u_{gl} - u^N)\|_{L^2(\Omega_{gl})}}{\|k^{1/2}\nabla u_{gl}\|_{L^2(\Omega_{gl})}} \leq \sqrt{2MM^*} \max_{i\in 1,\ldots,m} \left( \frac{C_2^2}{\text{diam}(\omega_i)^2} C_{Q,i}^2 + C_1^2 \right)^{1/2} \varepsilon_i. \tag{SM5.12}$$

The constant $C_Q$ can be calculated using an eigenvalue problem, all constants $C_{Q,i}$ for Example 1 are in the interval $(0.06, 0.13)$, for Example 2 they are in the interval $(0.06, 14)$ (use `4_4/calculate_cq.py` to reproduce).

For our examples, the constant $M$ has the value of 4, the constant $M^*$ has the value of 16, the constant $C_1$ has the value of 1, the constant $C_2/\text{diam}(\omega_i)$ has the value of $10 \cdot \sqrt{2}$.

Lemma SM5.2. *Let the reduced space $R_i^n$ associated with $\omega_i$ satisfy*

$$\left\|T_i - P_{R_i^n} T_i\right\| = \sup_{w\in S_i} \inf_{v\in R_i^n} \frac{\|T_i w - v\|_{R_i}}{\|w\|_{S_i}} \leq \frac{\varepsilon_i}{C_{S,i}}, \tag{SM5.13}$$

*where $C_{S,i}$ is the constant in the inequality $\|v|_{\Gamma_{out,i}}\|_{S_i} \leq C_{S,i}\|k^{1/2}\nabla v\|_{L^2(\omega_i^*)}$ for all $v \in H^1(\omega_i^*)/\mathbb{R}$ for subdomains $\omega_i^*$ with $\partial\omega_i^* \cap \Sigma_D = \emptyset$ or $v \in \{w \in H^1(\omega_i^*) : w = 0$ on $\Sigma_D \cap \partial\omega_i^*\}$. Then there exist $w_i \in R_i^n$ so that for $v_i := w_i + u_i^f|_{\omega_i}$ (SM5.8) holds.*

*Proof.* We show the result for subdomains that satisfy $\partial\omega_i^* \cap \Sigma_D = \emptyset$, noting that the proof for subdomains that border $\Sigma_D$ is slightly easier.

We split the local solution $u_{gl}|_{\omega_i^*}$ into three parts: First, we split it into two parts $u_{gl}|_{\omega_i^*} = u_i^f + u_i^\Gamma$ where $u_i^f$ solves

$$\mathcal{A}u^f = f \quad \text{in } \mathcal{X}_0',$$

and $u_i^\Gamma$ is the unique solution of the problem: Find $u_i^\Gamma \in \{v \in H^1(\omega_i^*) : v = u_{gl}$ on $\Gamma_{out,i},\ v = 0$ on $\Sigma_D \cap \partial\omega_i^*\}$ such that

$$Au_i^\Gamma = 0 \qquad \text{in } X_0'. \tag{SM5.14}$$

Then we further split $u_i^\Gamma = u_i^0 + a_{c,i}$ where $u_i^0 := u_i^\Gamma - |\omega_i^*|^{-1}\int_{\omega_i^*} u_i^\Gamma$ has mean value zero and $a_{c,i}$ is a constant function. Note that it holds $u_i^0|_{\omega_i} = T_i(u_i^0|_{\Gamma_{out,i}})$. We

choose $w_i$ to be the best approximation of $u_i^0$ in $R_i^n$. We obtain

$$\begin{aligned}\|k^{1/2}\nabla(u_{gl}-v_i)\|_{L^2(\omega_i)} &= \|k^{1/2}\nabla(u_i^f+u_i^\Gamma-u_i^f|_{\omega_i}-w_i)\|_{L^2(\omega_i)}\\ &= \|k^{1/2}\nabla(u_i^\Gamma-w_i)\|_{L^2(\omega_i)} = \|k^{1/2}\nabla(u_i^0-w_i)\|_{L^2(\omega_i)}\\ &= \left\|u_i^0-w_i\right\|_{R_i} \overset{\text{(SM5.13)}}{\leq} \frac{\varepsilon_i}{C_{S,i}}\|u_i^0|_\Gamma\|_{S_i}\\ &\leq \frac{\varepsilon_i}{C_{S,i}}C_{S,i}\|k^{1/2}\nabla u_i^0\|_{L^2(\omega_i^*)} = \varepsilon_i\|k^{1/2}\nabla u_i^\Gamma\|_{L^2(\omega_i^*)}.\end{aligned}$$

As $u_i^\Gamma$ solves (SM5.14), we may invoke the Lax-Milgram Lemma to infer

$$\begin{aligned}\|k^{1/2}\nabla u_i^\Gamma\|^2_{L^2(\omega_i^*)} &= \int_{\omega_i^*} k|\nabla u_i^\Gamma|^2\\ &= \min\left\{\int_{\omega_i^*} k|\nabla v|^2 \,:\, v\in H^1(\omega_i^*), v|_{\Gamma_{out}} = u_i^\Gamma|_{\Gamma_{out,i}}\right\}.\end{aligned}$$

Therefore, there holds

(SM5.15)
$$\|k^{1/2}\nabla u_i^\Gamma\|_{L^2(\omega_i^*)} \leq \|k^{1/2}\nabla v\|_{L^2(\omega_i^*)} \text{ for all } v\in H^1(\omega_i^*) \text{ satisfying } v|_{\Gamma_{out,i}} = u_i^\Gamma|_{\Gamma_{out,i}}.$$

As $u_i^f$ has zero trace on $\Gamma_{out,i}$ we may exploit (SM5.15) to conclude

$$\begin{aligned}\|k^{1/2}\nabla(u_{gl}-v_i)\|_{L^2(\omega_i)} &\leq \varepsilon_i\|k^{1/2}\nabla u_i^\Gamma\|_{L^2(\omega_i^*)}\\ &\leq \varepsilon_i\|k^{1/2}\nabla(u_i^\Gamma+u_i^f)\|_{L^2(\omega_i^*)} = \varepsilon_i\|k^{1/2}\nabla u_{gl}\|_{L^2(\omega_i^*)}.\end{aligned}$$

□

The constants $C_{S,i}$ are calculated using a localized eigenvalue problem, all constants $C_{S,i}$ for our GFEM examples are in the interval $(0.4, 1)$
(use `4_4/calculate_csi.py` to reproduce).

COROLLARY SM5.3. *Let all local reduced spaces $R_i^n$ satisfy SM5.13. Let further $u_i^f|_{\omega_i}$ be in $R_i^n$ for all $i$. Let further the constant function be in $R_i^n$ for all $i$ with $\partial\omega_i\cap\Sigma_D=\emptyset$. Then for the GFEM solution $u_{\text{GFEM}}$ it holds*
(SM5.16)
$$\frac{\|k^{1/2}\nabla(u_{gl}-u_{\text{GFEM}})\|_{L^2(\Omega_{gl})}}{\|k^{1/2}\nabla u_{gl}\|_{L^2(\Omega_{gl})}} \leq \sqrt{2MM^*}\max_{i\in 1,\dots,m}\left(\frac{C_2^2}{\text{diam}(\omega_i)^2}C_{p,f,i}^2\frac{k_1}{k_0}+C_1^2\right)^{1/2}\varepsilon_i.$$

*Proof.* Under the given assumptions, the function $u_N$ as defined in Proposition SM5.1 is in $X_{\text{GFEM}}$. The claim then follows directly from the Lemma of Céa.
□

Choosing the tolerances $\varepsilon_i$ as

$$\varepsilon_i = \texttt{tol}_{\text{GFEM}}\left[(2MM^*)\left(\left(\frac{C_2}{\text{diam}(\omega_i)}\right)^2 C_{Q,i}^2 + C_1^2\right)\right]^{-\frac{1}{2}} \tag{SM5.17}$$

leads to

$$\frac{\|k^{1/2}\nabla(u_{gl}-u_{\text{GFEM}})\|_{L^2(\Omega_{gl})}}{\|k^{1/2}\nabla u_{gl}\|_{L^2(\Omega_{gl})}} \leq \texttt{tol}_{\text{GFEM}}. \tag{SM5.18}$$

**SM6. Computation of singular values.** The singular values $\sigma_i$ of the operator $T$ can be calculated as the square root of the eigenvalues of the eigenvalue problem (2.14). However, solving this eigenvalue problem in 64bit floating point accuracy only yields the eigenvalues down to a relative size $\lambda_i/\lambda_1$ of about $10^{-16}$. This translates to a relative size of the singular values $\sigma_i/\sigma_1$ of about $10^{-8}$. To compute the singular values of relative size smaller than $10^{-8}$ in §4.1 and §4.4, we resorted to solving the eigenvalue problem: Find $\underline{\zeta}_i \in \mathbb{R}^{N_S+N_R}$ and $\lambda_i \in \mathbb{R}_0^+$ such that

$$\begin{pmatrix} 0 & \underline{T} \\ \underline{M}_S^{-1}\underline{T}^t\underline{M}_R & 0 \end{pmatrix} \underline{\zeta}_i = \lambda_i \underline{\zeta}_i. \tag{SM6.1}$$

The positive spectrum of this eigenvalue problem coincides with the singular values of the operator $T$, see e.g. [SM3, Chapter 8.6]. Recall that $\underline{M}_S^{-1}\underline{T}^t\underline{M}_R$ is the matrix representation of the adjoint operator $T^*$.

REFERENCES

[SM1] Z. Chen and J. J. Dongarra, *Condition numbers of Gaussian random matrices*, SIAM J. Matrix Anal. Appl., 27 (2005), pp. 603–620.

[SM2] M. Giaquinta and L. Martinazzi, *An introduction to the regularity theory for elliptic systems, harmonic maps and minimal graphs*, vol. 11 of Appunti. Scuola Normale Superiore di Pisa (Nuova Serie) [Lecture Notes. Scuola Normale Superiore di Pisa (New Series)], Edizioni della Normale, Pisa, second ed., 2012.

[SM3] G. H. Golub and C. F. Van Loan, *Matrix computations*, vol. 3, Johns Hopkins University Press, Baltimore, MD, 2012.

[SM4] Y. Gordon, *Some inequalities for Gaussian processes and applications*, Israel J. Math., 50 (1985), pp. 265–289.

[SM5] Y. Gordon, *Gaussian processes and almost spherical sections of convex bodies*, Ann. Probab., 16 (1988), pp. 180–188.

[SM6] N. Halko, P.-G. Martinsson, and J. A. Tropp, *Finding structure with randomness: Probabilistic algorithms for constructing approximate matrix decompositions*, SIAM Rev., 53 (2011), pp. 217–288.

[SM7] J. M. Melenk and I. Babuška, *The partition of unity finite element method: basic theory and applications*, Comput. Methods Appl. Mech. Engrg., 139 (1996), pp. 289–314.

[SM8] T. Taddei, *Model order reduction methods for data assimilation; state estimation and structural health monitoring*, PhD thesis, Massachusetts Insitute of Technology, 2016.
